# Supplementary material for: Is Externally Corrected Coupled Cluster Always Better than the Underlying Truncated Configuration Interaction?
Source: arXiv:2102.10143 ancillary file (2021-05-28)
Supplement: Supplementary file 1 [file ec-CC_SI.pdf]

# Supporting information for:
# Is Externally Corrected Coupled Cluster Always Better than the Underlying Truncated Configuration Interaction?

Ilias Magoulas,[†] Karthik Gururangan,[†] Piotr Piecuch,[*,†,‡] J. Emiliano Deustua,[†] and Jun Shen[†]

†*Department of Chemistry, Michigan State University, East Lansing, Michigan 48824, USA*

‡*Department of Physics and Astronomy, Michigan State University, East Lansing, Michigan 48824, USA*

E-mail: piecuch@chemistry.msu.edu

This Supporting Information document reports the results of the numerical experiment in which we allowed the CIPSI algorithm, as implemented in Quantum Package 2.0, adopted in our ec-CC computations, to grow the Hamiltonian diagonalization spaces $\mathcal{V}_{\text{int}}$ more rapidly compared to the default dimension-doubling mechanism discussed in the main text. As in Sections 2.2 and 3, our test case was the water molecule, as described by the cc-pVDZ basis set, in which we correlated all electrons. Since our main observations, discussed below, do not depend on the nuclear geometry, in presenting our results, we focus on the $R = 2R_e$ structure, in which both O–H bonds are stretched by a factor of 2 and which is located between the weakly correlated (in this study, $R = R_e$) and strongly correlated (in this study, $R = 3R_e$) regions. In carrying out our numerical experiment, we fixed the wave function termination input parameter $N_{\text{det(in)}}$ used by CIPSI at 100,000 and considered several values of the parameter $f$, which controls the growth of the $\mathcal{V}_{\text{int}}$ spaces in each CIPSI run, greater than the $f = 2$ default. We chose $N_{\text{det(in)}} = 100,000$, since when $f$ is considerably larger than 2, the $\mathcal{V}_{\text{int}}$ growth algorithm of CIPSI reaches the $N_{\text{det(in)}}$ values smaller than 100,000 too rapidly to draw meaningful conclusions. At the same time, when $N_{\text{det(in)}}$ becomes significantly larger than 100,000, the CIPSI and CIPSI-based ec-CC energies for the $H_2O$/cc-pVDZ system are too close to FCI to learn anything useful. For the completeness of our analysis, we also considered a few values of $f$ between 1 and 2, slowing down the growth of the CIPSI wave functions compared to the $f = 2$ default even further at the expense of increasing the number of diagonalizations needed to exceed $N_{\text{det(in)}}$. As in the case of the calculations shown in Table 2 of the main text, all CIPSI runs reported in this Supporting Information were initiated from the RHF wave function.

The results of our numerical test, in which we cluster analyzed the final CIPSI wave functions obtained for the $R = 2R_e$ $H_2O$/cc-pVDZ system using $N_{\text{det(in)}} = 100,000$ and several values of $f$ ranging from 1.05 to 10, employing the resulting $T_3$ and $T_4$ amplitudes in the subsequent ec-CC-I, ec-CC-II, and ec-CC-II$_3$ calculations, are summarized in Table S1. As in Table 2 in the main text, in addition to the ec-CC-I, ec-CC-II, and ec-CC-II$_3$ energies

and the variational ($E_{\text{var}}$) and perturbatively corrected ($E_{\text{var}} + \Delta E^{(2)}$ and $E_{\text{var}} + \Delta E_r^{(2)}$) CIPSI data, we show the percentages of the singly, doubly, triply, and quadruply excited $S_z = 0$ determinants of $A_1$ symmetry captured during the CIPSI computations and the total numbers of determinants defining the final Hamiltonian diagonalization spaces $\mathcal{V}_{\text{int}}$ of the CIPSI runs shown in Table S1, designated as $N_{\text{det(out)}}$. As explained in the main text, each CIPSI calculation consists of multiple steps, called CIPSI iterations, where a single CIPSI iteration involves the diagonalization of the Hamiltonian in the current space $\mathcal{V}_{\text{int}}$, resulting in the wave function abbreviated in the main text as $|\Psi^{(\text{CIPSI})}\rangle$, and the identification of the $\mathcal{V}_{\text{ext}}$ space associated with $|\Psi^{(\text{CIPSI})}\rangle$, needed to construct $\mathcal{V}_{\text{int}}$ for the subsequent diagonalization. Thus, in addition to the dimensions $N_{\text{det(out)}}$ characterizing the final diagonalization spaces $\mathcal{V}_{\text{int}}$, we provide information about the numbers of CIPSI iterations, denoted as $N_{\text{diag}}$, required to complete the CIPSI runs reported in Table S1.

In analogy to the calculations presented in Table 2 of the main text, the sequence of Hamiltonian diagonalizations characterizing each CIPSI run was terminated when the dimension of space $\mathcal{V}_{\text{int}}$ exceeded $N_{\text{det(in)}}$ (which is why $N_{\text{det(out)}}$ is always greater than $N_{\text{det(in)}}$). There is, however, a difference between the CIPSI and ec-CC computations reported in Tables 2 and S1. In the case of Table 2, we kept the input parameter $f$ at its default value of 2 and varied $N_{\text{det(in)}}$. In the case of the CIPSI and CIPSI-based ec-CC calculations shown in Table S1, we fixed $N_{\text{det(in)}}$ at 100,000 and varied $f$ to examine the impact of the rate of the growth of the CIPSI wave functions on the ec-CC, especially ec-CC-II and ec-CC-II$_3$, data. We will not comment on the ec-CC-I results, since, in agreement with the formal considerations and numerical evidence presented in the main text, once the underlying CIPSI calculations capture all or nearly all singly and doubly excited determinants, as is the case in all CIPSI runs reported in Table S1, the CIPSI-based ec-CC-I and variational CIPSI ($E_{\text{var}}$) energies become identical or nearly identical.

While the significance of the various combinations of the input parameters $f$ and $N_{\text{det(in)}}$ used by CIPSI for the quality of the ec-CC-II and ec-CC-II$_3$ energies requires a more thorough

examination involving several molecules of varying size and larger basis sets, which is outside the scope of the present study, the results in Table S1 indicate that just like the CIPSI calculations themselves, the ec-CC-II and ec-CC-II$_3$ schemes benefit from a tempered growth of the CIPSI wave function achieved by using $f$ around 2. One might argue that using the values of $f$ slightly larger than 2, such as $f = 3$, which has a minimal effect on the ec-CC-II and ec-CC-II$_3$ energies and the final wave function size $N_{\text{det(out)}}$, while reducing the number of Hamiltonian diagonalizations in the CIPSI run from 15, when $f = 2$, to 10, is better than the $f = 2$ default adopted by Quantum Package 2.0, and we will return to such detailed analyses in our future work, but it is clear from Table S1 that one should avoid growing the CIPSI wave functions too rapidly.

Indeed, when $f$ is considerably greater than 2, two types of situations – none benefiting CIPSI and the associated ec-CC-II and ec-CC-II$_3$ calculations – can occur. In the first category of situations that can emerge in the CIPSI and CIPSI-based ec-CC runs with $f \gg 2$, illustrated in Table S1 by the $f = 6$ and 9 data, the dimension of the final CIPSI diagonalization space, $N_{\text{det(out)}}$, becomes much larger than the wave function termination input parameter $N_{\text{det(in)}}$. This happens when the dimension of the $\mathcal{V}_{\text{int}}$ space used in the CI calculation immediately prior to the final CIPSI iteration is only slightly smaller than $N_{\text{det(in)}}$. In situations like this, the final Hamiltonian diagonalization of a given CIPSI run, preceding the ec-CC steps, becomes much more expensive than its $f = 2$ counterpart using the same $N_{\text{det(in)}}$ value, while offering relatively small improvements in the variational and perturbatively corrected CIPSI data and the resulting ec-CC-II and ec-CC-II$_3$ energies, which can be improved a lot more substantially by increasing $N_{\text{det(in)}}$ and slowing down the wave function growth.

Let us, for example, compare the $E_{\text{var}}$, $E_{\text{var}} + \Delta E^{(2)}$ or $E_{\text{var}} + \Delta E_r^{(2)}$, ec-CC-II, and ec-CC-II$_3$ energies obtained for the $H_2O$/cc-pVDZ molecule at $R = 2R_e$ using $N_{\text{det(in)}} = 100,000$ and $f = 9$, shown in Table S1, with the analogous energy values produced in the $N_{\text{det(in)}} = 500,000$, $f = 2$ calculations, reported in Table 2 of the main text, which

result in a similarly large $N_{\text{det(out)}}$ dimension (as in the main text, when commenting on the perturbatively corrected CIPSI energies, we focus on the $E_{\text{var}} + \Delta E^{(2)}$ values, which are nearly identical to their $E_{\text{var}} + \Delta E_r^{(2)}$ counterparts). The final CIPSI diagonalization space obtained with $N_{\text{det(in)}} = 100,000$ and $f = 9$ has a dimension $N_{\text{det(out)}} = 629,647$, which is much larger than the wave function termination input parameter $N_{\text{det(in)}}$ used to generate it. This is because the dimension of the $\mathcal{V}_{\text{int}}$ space characterizing the previous Hamiltonian diagonalization of the same CIPSI run, of 70,143, while being less than $N_{\text{det(in)}} = 100,000$, is quite close to it, making the length of the final CIPSI wave function vector, which is, more or less, $f$ times 70,143, much larger than the associated $N_{\text{det(in)}}$ value when $f = 9$. The final CIPSI state characterized by $N_{\text{det(out)}} = 629,647$, obtained using $N_{\text{det(in)}} = 100,000$ and a rapid wave function growth defined by $f = 9$, improves the variational and perturbatively corrected CIPSI and ec-CC-II and ec-CC-II$_3$ calculations compared to the $N_{\text{det(in)}} = 100,000$, $f = 2$ CIPSI run, in which the final $\mathcal{V}_{\text{int}}$ dimension is about 3.5 times smaller, reducing the 1.418, 0.046, 0.467, and 0.356 millihartree errors relative to FCI characterizing the $E_{\text{var}}$, $E_{\text{var}} + \Delta E^{(2)}$, ec-CC-II, and ec-CC-II$_3$ energies obtained with $N_{\text{det(in)}} = 100,000$ and $f = 2$ to 0.890, 0.019, 0.336, and 0.281 millihartree, respectively, but we must keep in mind that the Hamiltonian diagonalization characterized by $N_{\text{det(out)}} = 629,647$ is much more expensive than its $f = 2$ counterpart using only 181,579 determinants. If one is interested in taking advantage of longer CI wave function expansions of the type obtained here with $N_{\text{det(in)}} = 100,000$ and $f = 9$ in the determination of the variational and perturbatively corrected CIPSI and ec-CC-II and ec-CC-II$_3$ energies, it is a lot better to use larger $N_{\text{det(in)}}$ values combined with a much slower wave function growth defined by $f$ around 2. Indeed, as shown in Table 2 of the main text, by choosing $N_{\text{det(in)}} = 500,000$ and $f = 2$ that result in the final CIPSI wave function size $N_{\text{det(out)}} = 718,316$, one reduces the 0.890, 0.019, 0.336, and 0.281 millihartree errors relative to FCI characterizing the $E_{\text{var}}$, $E_{\text{var}} + \Delta E^{(2)}$, ec-CC-II, and ec-CC-II$_3$ energies obtained with $N_{\text{det(in)}} = 100,000$ and $f = 9$, which produce a similarly large $N_{\text{det(out)}}$ value of 629,647, to as little as 0.273, 0.009, 0.147, and 0.138 millihartree,

respectively. It should also be noted that the final CIPSI wave functions resulting from the $N_{\text{det(in)}} = 500,000$, $f = 2$ and $N_{\text{det(in)}} = 100,000$, $f = 9$ calculations, in addition to having similar $N_{\text{det(out)}}$ lengths, capture the nearly identical fractions of the singly, doubly, triply, and quadruply excited determinants, but the CIPSI and CIPSI-based ec-CC energies obtained with $N_{\text{det(in)}} = 100,000$ and $f = 9$, where the underlying CI wave function is grown rapidly, are considerably worse than their counterparts produced using $N_{\text{det(in)}} = 500,000$ and a tempered-growth mechanism defined by $f = 2$. A tempered wave function growth via multiple Hamiltonian diagonalizations in slowly increasing $\mathcal{V}_{\text{int}}$ spaces allows the CIPSI algorithm to carefully probe the many-electron Hilbert space and optimize the CI expansion coefficients more accurately, resulting in a higher-quality final CI state that improves the accuracy of the variational and perturbatively corrected CIPSI energies and their ec-CC-II and ec-CC-II$_3$ counterparts without making the corresponding CI expansion much longer.

Similar remarks apply to a comparison of the $N_{\text{det(in)}} = 100,000$ calculations characterized by the rapid wave function growth defined by $f = 6$, which results in a large $N_{\text{det(out)}}$ value of 451,030, with the $N_{\text{det(in)}} = 500,000$, $f = 2$ CIPSI and ec-CC runs that rely on a substantially slower growth of the $\mathcal{V}_{\text{int}}$ space and a final CI state with $N_{\text{det(out)}} = 718,316$. When $N_{\text{det(in)}} = 100,000$ and $f = 6$, the $\mathcal{V}_{\text{int}}$ space characterizing the CIPSI iteration immediately prior to the final Hamiltonian diagonalization is 75,308, i.e., it is again quite close to the wave function termination input parameter $N_{\text{det(in)}}$, so that one ends up with the CI wave function expansion about 4.5 times longer than $N_{\text{det(in)}}$. This reduces the 1.418, 0.046, 0.467, and 0.356 millihartree errors relative to FCI characterizing the $E_{\text{var}}$, $E_{\text{var}} + \Delta E^{(2)}$, ec-CC-II, and ec-CC-II$_3$ energies obtained with $N_{\text{det(in)}} = 100,000$ and $f = 2$, but the resulting error values, of 1.189, 0.024, 0.398, and 0.305 millihartree, respectively, are not substantially smaller than those obtained using the much more compact final CI wave function generated in the $N_{\text{det(in)}} = 100,000$, $f = 2$ CIPSI run, where $N_{\text{det(out)}}$ is only 181,579. At the same time, the errors in the $E_{\text{var}}$, $E_{\text{var}} + \Delta E^{(2)}$, ec-CC-II, and ec-CC-II$_3$ energies relative to the corresponding FCI data resulting from the $N_{\text{det(in)}} = 100,000$,

$f = 6$ CIPSI run are 2.2–4.4 times larger than those obtained in the $N_{\text{det(in)}} = 500,000$, $f = 2$ computations, in which the underlying Hamiltonian diagonalization spaces $\mathcal{V}_{\text{int}}$ are grown a lot more slowly without making the final $N_{\text{det(out)}}$ dimension much larger. This reaffirms our previous observations based on comparing the $N_{\text{det(in)}} = 100,000$, $f = 9$ and $N_{\text{det(in)}} = 500,000$, $f = 2$ CIPSI and CIPSI-based ec-CC runs.

In the second category of situations that may occur when $f$ is significantly larger than the default value of 2, the final CIPSI wave functions, which enter the ec-CC considerations, are characterized by dimensions $N_{\text{det(out)}}$ that are similar to or not much greater than the wave function termination input parameter $N_{\text{det(in)}}$. This happens when the dimension of the $\mathcal{V}_{\text{int}}$ space used in the CI calculation immediately prior to the final Hamiltonian diagonalization of a given CIPSI run is so much smaller than $N_{\text{det(in)}}$ that one needs an extra CIPSI iteration to produce the $\mathcal{V}_{\text{int}}$ space larger than $N_{\text{det(in)}}$. In situations like this, the final Hamiltonian diagonalization of a given CIPSI run, preceding the ec-CC steps, has computational costs similar to those characterizing the $f = 2$ calculations using the same $N_{\text{det(in)}}$, but since the final $\mathcal{V}_{\text{int}}$ space used by CIPSI is reached very rapidly when $f$ is much larger than 2, generating a CI state of relatively low quality, the resulting variational and perturbatively corrected CIPSI energies and their ec-CC-II and ec-CC-II$_3$ counterparts are substantially worse than those obtained with $f = 2$.

In the case of the calculations for the $H_2O$/cc-pVDZ molecule at $R = 2R_e$ using $N_{\text{det(in)}} = 100,000$, shown in Table S1, examples that illustrate the above statements best are the CIPSI and ec-CC runs corresponding to $f = 7$ and 10. In both of these cases, the $N_{\text{det(out)}}$ dimensions of the final CIPSI diagonalization spaces, which are 182,202 for $f = 7$ and 105,624 for $f = 10$, are not much larger than the wave function termination input parameter $N_{\text{det(in)}}$, but since these spaces are reached rapidly, in only a few CIPSI iterations, the resulting CI states and the corresponding variational and perturbatively corrected CIPSI energies and their ec-CC-II and ec-CC-II$_3$ counterparts are of considerably lower quality than those obtained in the analogous $f = 2$ computations. We can see this by comparing the $E_{\text{var}}$,

$E_{\text{var}} + \Delta E^{(2)}$, ec-CC-II, and ec-CC-II$_3$ energies obtained with $N_{\text{det(in)}} = 100,000$ and $f = 7$ with the analogous energy values produced using the same $N_{\text{det(in)}}$ and $f = 2$, shown in Table S1. Both sets of calculations are characterized by the nearly identical dimensions $N_{\text{det(out)}}$, of 182,202 in the $f = 7$ case and 181,579 when $f = 2$, and very similar fractions of the singly, doubly, triply, and quadruply excited determinants captured by the respective CIPSI runs. However, the 2.277, 0.073, 0.631, and 0.440 millihartree errors relative to FCI characterizing the $E_{\text{var}}$, $E_{\text{var}}+\Delta E^{(2)}$, ec-CC-II, and ec-CC-II$_3$ energies, respectively, obtained with $N_{\text{det(in)}} = 100,000$ and $f = 7$, where the underlying CI wave function is grown rapidly (the dimension of the $\mathcal{V}_{\text{int}}$ space immediately prior to the final Hamiltonian diagonalization is only 26,055), are substantially larger than the 1.418, 0.046, 0.467, and 0.356 millihartree errors obtained using a tempered-growth mechanism enforced by choosing $f = 2$. The worsening of the $E_{\text{var}}$, $E_{\text{var}} + \Delta E^{(2)}$, ec-CC-II, and ec-CC-II$_3$ energies as a result of growing the CIPSI wave function too rapidly becomes even more apparent when $f = 10$. In this case, the dimension of the final diagonalization space $\mathcal{V}_{\text{int}}$, of 105,624, is even closer to $N_{\text{det(in)}}$ than in the case of the $f = 7$ CIPSI run, but because this space is reached very fast, in only five CIPSI iterations (the $\mathcal{V}_{\text{int}}$ space immediately prior to the final Hamiltonian diagonalization has only 10,562 determinants), the quality of the $E_{\text{var}}$, $E_{\text{var}} + \Delta E^{(2)}$, ec-CC-II, and ec-CC-II$_3$ energies, which differ from their FCI counterpart by 3.404, 0.094, 0.954, and 0.562, respectively, is much lower than that resulting from using $f = 2$, where the corresponding errors are about twice as small.

Since growing the CIPSI wave function too fast does not benefit the ec-CC-II and ec-CC-II$_3$ calculations, let us examine if slowing down the wave function growth compared to the $f = 2$ default even further by considering the $f$ values between 1 and 2 can help. As shown in Table S1, choosing the values of $f$ close to 1, such as 1.25 or 1.05, which allow the final CIPSI iterations to accumulate higher-order correlation effects in compact wave functions characterized by the $N_{\text{det(out)}}$ dimensions only slightly larger than $N_{\text{det(in)}}$, does not have a significant effect on the quality of the ec-CC-II and ec-CC-II$_3$ energies obtained

using $f = 2$, while increasing the computational costs due to large numbers of Hamiltonian diagonalizations required by the very slowly growing $\mathcal{V}_{\text{int}}$ spaces in the underlying CIPSI runs. The CIPSI results, especially the final $E_{\text{var}} + \Delta E^{(2)}$ values, do not improve either.

Let us, for example, compare the $E_{\text{var}}$, $E_{\text{var}} + \Delta E^{(2)}$, ec-CC-II, and ec-CC-II$_3$ energies of the $R = 2R_e$ $H_2O$/cc-pVDZ system obtained using $N_{\text{det(in)}} = 100,000$ and $f = 1.25$ with their counterparts resulting from the CIPSI and ec-CC calculations using the same $N_{\text{det(in)}}$ and $f = 2$. The final CIPSI wave function generated in the $N_{\text{det(in)}} = 100,000$, $f = 1.25$ run, characterized by $N_{\text{det(out)}} = 111,189$, is indeed very compact, containing enough high-order information to reduce the 1.418 millihartree error relative to FCI characterizing the variational CIPSI energy $E_{\text{var}}$ obtained using $f = 2$ to 1.366 millihartree, but neither the perturbatively corrected $E_{\text{var}} + \Delta E^{(2)}$ value nor the corresponding ec-CC-II and ec-CC-II$_3$ energies substantially change compared to the $f = 2$ calculations using the same $N_{\text{det(in)}}$. The $E_{\text{var}} + \Delta E^{(2)}$ and ec-CC-II energies slightly worsen, by 0.013 and 0.036 millihartree, respectively, and the ec-CC-II$_3$ energy minimally improves, by 0.004 millihartree, i.e., the results of the perturbatively corrected CIPSI computations and their ec-CC-II and ec-CC-II$_3$ counterparts change very little, but the number of Hamiltonian diagonalizations involved in the underlying CIPSI runs increases quite dramatically when the dimension-doubling mechanism is replaced by the even slower wave function growth defined by $f = 1.25$, from 15, when $f = 2$, to 37 when $f = 1.25$. The $N_{\text{det(in)}} = 100,000$, $f = 1.05$ calculations, which produce an even more compact CIPSI wave function with the $N_{\text{det(out)}}$ value almost identical to $N_{\text{det(in)}}$, reduce the 1.418 millihartree error relative to FCI characterizing the variational CIPSI energy $E_{\text{var}}$ obtained with $f = 2$ to 1.198 millihartree, which is a more substantial improvement compared to $f = 1.25$, but this does not translate into similar improvements in the $E_{\text{var}} + \Delta E^{(2)}$, ec-CC-II, and ec-CC-II$_3$ energies. The $E_{\text{var}} + \Delta E^{(2)}$ energy obtained using $f = 1.05$ slightly worsens compared to its $f = 2$ counterpart (by 0.002 millihartree), whereas the ec-CC-II and ec-CC-II$_3$ results improve only very little, reducing the 0.467 and 0.356 millihartree errors relative to FCI obtained with $f = 2$ to 0.454 and

0.296 millihartree, respectively, when the $f = 1.05$ value is employed. At the same time, the number of Hamiltonian diagonalizations needed to complete the $N_{\text{det(in)}} = 100,000$, $f = 1.05$ CIPSI run is 146, as opposed to only 15 required by its $f = 2$ counterpart, making the calculations much more expensive. They are not only considerably more expensive due to the increase in the number of diagonalizations by a factor of about 10, but also because the dimensions of many $\mathcal{V}_{\text{int}}$ spaces preceding the final CIPSI iteration are close to $N_{\text{det(out)}}$ or the wave function termination input parameter $N_{\text{det(in)}}$ when $f$ is as small as 1.05. For example, the dimensions of the last five $\mathcal{V}_{\text{int}}$ spaces defining the $N_{\text{det(in)}} = 100,000$, $f = 1.05$ run, starting with the final $N_{\text{det(out)}}$ value, are 103,788, 98,846, 94,136, 89,641, and 85,369. This should be compared to the much more rapidly decaying dimensions of the last five $\mathcal{V}_{\text{int}}$ spaces characterizing the $N_{\text{det(in)}} = 100,000$, $f = 2$ run, which are 181,579, 90,880, 45,436, 22,701, and 11,350, respectively.

Given the very small effect of replacing the $f = 2$ value by the values of $f$ between 1 and 2 on the ec-CC-II and ec-CC-II$_3$ energies, and the fact that the CIPSI runs using $f$ close to 1 result in large numbers of Hamiltonian diagonalizations that can be substantially more expensive than those encountered in the $f = 2$ calculations, we see no advantages in slowing down the wave function growth beyond the default dimension-doubling mechanism adopted by the implementation of CIPSI in Quantum Package 2.0. Again, one might try to argue that the intermediate values of $f$ between 1 and 2, such as $f = 1.5$, could be a good compromise, since the increase in the number of Hamiltonian diagonalizations required by CIPSI is relatively modest when $f = 2$ is replaced by $f = 1.5$, and very few of them have dimensions closer to $N_{\text{det(in)}}$, but, as shown in Table S1, the $E_{\text{var}} + \Delta E^{(2)}$, ec-CC-II, and ec-CC-II$_3$ energies do not improve when the default dimension-doubling mechanism is replaced by the somewhat slower growth defined by $f = 1.5$.

Based on the preliminary analysis reported in this Supporting Information document, the default dimension-doubling mechanism adopted in the implementation of CIPSI in Quantum Package 2.0, which enforces the much desired tempered growth of the CI wave functions

employed in the subsequent ec-CC runs without making the calculations too expensive, is a good choice. There may be situations where using the values of the input parameter $f$ slightly larger than 2, such as 3 or 4, can offer further help by reducing the number of Hamiltonian diagonalizations in the CIPSI runs, while maintaining the accuracy of the ec-CC-II and ec-CC-II$_3$ energies obtained with $f = 2$, but adopting the $f = 2$ default is certainly reasonable. While it is already quite clear that neither the rapid growth of the CIPSI wave functions by using the values of $f$ much larger than 2 nor the ultra-slow wave function growth corresponding to $f$ only slightly above 1 benefit the CIPSI-based ec-CC-II and ec-CC-II$_3$ computations, a thorough investigation of the significance of the various choices of the input parameters $f$ and $N_{\text{det(in)}}$ used by CIPSI for the quality of the ec-CC-II and ec-CC-II$_3$ energies is worth pursuing. Since such an investigation, which requires testing many molecules and basis sets of varying size and larger numbers of nuclear geometries, is outside the scope of the present study, we will return to this issue in the future work.

Table S1: The results of the all-electron CIPSI calculations, initiated from the RHF wave function, and of the corresponding CIPSI-driven ec-CC computations for the stretched, $R = 2R_e$, structure of the $H_2O$ molecule, as described by the cc-pVDZ basis set, in which the wave function termination input parameter $N_{\text{det(in)}}$ employed by the CIPSI algorithm was fixed at 100,000 and the parameter $f$ that controls the growth of the Hamiltonian diagonalization spaces $\mathcal{V}_{\text{int}}$ in each CIPSI run was allowed to vary from 1.05 to 10.

| $f$ | $N_{\text{det(out)}}$ | $N_{\text{diag}}$[a] | %S[b] | %D[b] | %T[b] | %Q[b] | CIPSI[c] | | | ec-CC[c] | | |
|---|---|---|---|---|---|---|---|---|---|---|---|---|
| | | | | | | | $E_{\text{var}}$ | $E_{\text{var}} + \Delta E^{(2)}$ | $E_{\text{var}} + \Delta E_r^{(2)}$ | I | II | $\text{II}_3$ |
| 1.05 | 103,788 | 146 | 87.9 | 83.8 | 21.4 | 4.2 | 1.198 | 0.048 | 0.049 | 1.195 | 0.454 | 0.296 |
| 1.25 | 111,189 | 37 | 93.9 | 86.8 | 23.5 | 4.4 | 1.366 | 0.059 | 0.059 | 1.364 | 0.503 | 0.352 |
| 1.5 | 139,131 | 24 | 97.0 | 90.1 | 28.0 | 5.5 | 1.392 | 0.053 | 0.053 | 1.391 | 0.516 | 0.395 |
| 2[d] | 181,579 | 15 | 100 | 91.6 | 31.7 | 6.8 | 1.418 | 0.046 | 0.046 | 1.417 | 0.467 | 0.356 |
| 3 | 208,298 | 10 | 100 | 91.3 | 32.9 | 7.8 | 1.637 | 0.064 | 0.064 | 1.636 | 0.482 | 0.349 |
| 4 | 155,352 | 8 | 100 | 90.1 | 28.5 | 5.8 | 2.181 | 0.080 | 0.081 | 2.179 | 0.543 | 0.315 |
| 5 | 157,758 | 7 | 100 | 88.6 | 27.9 | 5.9 | 2.159 | 0.066 | 0.067 | 2.152 | 0.604 | 0.393 |
| 6 | 451,030 | 7 | 100 | 96.3 | 45.4 | 15.2 | 1.189 | 0.024 | 0.024 | 1.189 | 0.398 | 0.305 |
| 7 | 182,202 | 6 | 100 | 90.6 | 30.5 | 7.0 | 2.277 | 0.073 | 0.074 | 2.273 | 0.631 | 0.440 |
| 8 | 344,528 | 6 | 100 | 94.0 | 42.3 | 11.8 | 1.278 | 0.045 | 0.045 | 1.277 | 0.447 | 0.332 |
| 9 | 629,647 | 6 | 100 | 98.0 | 53.1 | 20.2 | 0.890 | 0.019 | 0.019 | 0.890 | 0.336 | 0.281 |
| 10 | 105,624 | 5 | 97.0 | 86.3 | 22.9 | 4.3 | 3.404 | 0.094 | 0.096 | 3.381 | 0.954 | 0.562 |

[a] The number of CIPSI iterations, each consisting of the diagonalization of the Hamiltonian in the current space $\mathcal{V}_{\text{int}}$ to determine $|\Psi^{(\text{CIPSI})}\rangle$ and the identification of the associated $\mathcal{V}_{\text{ext}}$ space needed to construct $\mathcal{V}_{\text{int}}$ for the subsequent CIPSI iteration. [b] %S, %D, %T, and %Q are, respectively, the percentages of the singly, doubly, triply, and quadruply excited $S_z = 0$ determinants of $A_1$ symmetry captured during the CIPSI computations. [c] Errors relative to FCI in millihartree (for the FCI energy at $R = 2R_e$, see Table 1 in the main text). [d] The default $f$ value in Quantum Package 2.0.
